# Supplementary material for: Bridging SFT and DPO for Diffusion Model Alignment with Self-Sampling Preference Optimization
Source: arXiv:2410.05255 source file (2025-07-01)
Supplement: Supplementary file 1 [file appendix_A.tex]

\section{Proof}

\subsection{Proof of \eqref{eq:prior_prob}}
\label{app:proof_prob_nike}

Optionally include supplemental material (complete proofs, additional experiments and plots) in appendix.
All such materials \textbf{SHOULD be included in the main submission.}
