# Supplementary material for: Bridging SFT and DPO for Diffusion Model Alignment with Self-Sampling Preference Optimization
Source: arXiv:2410.05255 source file (2025-07-01)
Supplement: Supplementary file 2 [file appendix_B.tex]

\section{Supplementary Experiments}
\label{app:Experiments}

\subsection{Supplementary Experimental Settings}
\label{sec:app_exp_setting}

We list hyperparameter details in the training process in Table \ref{table:hyper}.
\begin{table}[t]
\caption{Hyperparameter Settings in MaPPO.}
\centering
 % \small
\label{table:hyper}
\begin{tabular}{c|cc}
\toprule[1.1pt]
% \hline
{Hyperparameter} & {Value} & {} \\
\midrule[1.1pt]
{batch size} & {$128$} & { } \\
{learning rate} & { } & { } \\
{optimizer} & {AdamW} & { } \\
{$\beta$} & { } & { } \\
{temperature} & {$1.0$} & { } \\
\bottomrule[1.1pt]
\end{tabular}
\end{table}

\subsection{Supplementary Results}
\label{app:supp_results}
